# Supplementary material for: Improving Diffusion Models for Authentic Virtual Try-on in the Wild
Source: arXiv:2403.05139 source file (2024-07-29)
Supplement: Supplementary file 1 [file furtherapp.tex]

\begin{figure}[ht]
    \small\centering
    \includegraphics[width=0.95\linewidth]{resources/appendix/further_exp.pdf}
    \vspace{-5pt}
    \caption{
    \textbf{Exemplar-based inpainting with \sname~when images are not from fashion domain.} We further investigate the potential of exemplar-based inpainting using \sname. Though \sname~is trained on garment-human pair data only, it generates authentic images with preserving details of reference images, even across different domains. We use the input images from Paint-by-Example~\cite{yang2023paint}.
    }
    \label{fig:furtherapp}
    \vspace{-10pt}
\end{figure}
